# Supplementary material for: Robust Evaluation of Diffusion-Based Adversarial Purification
Source: arXiv:2303.09051 source file (2023-12-03)
Supplement: Supplementary file 2 [file best_other_attacks.tex]

\begin{table}[!ht]
    \centering
    \begin{tabular}{lc}
    \toprule
        Attack & Robust Accuracy (\%) \\ \midrule
        Square~\citep{Andriushchenko2019SquareAA} & 89.38±0.26 \\
        FAB~\citep{Croce2019MinimallyDA} & 89.18±0.60 \\
        Deep Fool~\citep{MoosaviDezfooli2015DeepFoolAS} & 82.32±0.14 \\
        FMN Attack~\citep{Pintor2021FastMA} & 80.86±1.80 \\ \bottomrule
    \end{tabular}
    \caption{Robust accuracy against several threat models $\ell_\infty (\epsilon = 8/255)$ on CIFAR-10. Square attack is a black-box attack, and the others are white-box attacks.}
    \label{table:best_other_attack}
\end{table}
