# Supplementary material for: Robust Evaluation of Diffusion-Based Adversarial Purification
Source: arXiv:2303.09051 source file (2023-12-03)
Supplement: Supplementary file 3 [file best_svhn.tex]

\begin{table}[!ht]
    \centering
    \begin{tabular}{ccccc}
        \toprule
        \multirow{2}{*}{Defense} & \multirow{2}{*}{Attack} & \multirow{2}{*}{Classifier} & \multicolumn{2}{c}{Accuracy (\%)} \\
         & & & Standard & Robust \\ \midrule
        \citet{Rade2022ReducingEM} & AutoAttack & ResNet-18 & 93.08 & 52.83 \\
        \citet{Gowal2020UncoveringTL} & AutoAttack & WRN-28-10 & 92.87 & 56.83 \\
        \citet{Gowal2021ImprovingRU} & AutoAttack & WRN-28-10 & 94.15 & 60.90 \\ \midrule
        \citet{Nie2022DiffusionMF} & PGD+EOT & WRN-28-10 & 97.85±0.53 & 34.30±0.41 \\
        Ours & PGD+EOT & WRN-28-10 & 95.55±0.40 & 49.65±1.06 \\ \bottomrule
    \end{tabular}
    \caption{Standard and robust accuracy against adversarial attacks $\ell_\infty (\epsilon = 8/255)$ on SVHN. We compare our performance with adversarial training defenses.}
    \label{table:best_svhn}
\end{table}
